# Supplementary material for: Focus: Querying Large Video Datasets with Low Latency and Low Cost
Source: arXiv:1801.03493 source file (2018-01-10)
Supplement: Supplementary file 1 [file appendix.tex]

\appendix
%\pagebreak
\section*{Appendix}
\section{Video Stream URLs}
\label{appendix:video_url}

Most of our video dataset are obtained from YouTube live
streams. Table~\ref{table:video_url} summarizes the URLs of the live
streams that are publicly available. 

\begin{table}[h]
\scriptsize \centering \caption{Video dataset URL}
\label{table:video_url}
\begin{tabular}{|l|l|} \hline

Name & URL \\ \hline

auburn\_c & \url{https://www.youtube.com/watch?v=yJAk_FozAmI} \\ \hline
auburn\_r & \url{https://www.youtube.com/watch?v=cjuskMMYlLA} \\ \hline
bend & \url{https://www.youtube.com/watch?v=SNz323Cyago} \\ \hline
jacksonh & \url{https://www.youtube.com/watch?v=psfFJR3vZ78} \\ \hline
church\_st & \url{https://www.youtube.com/watch?v=S3Bl8AuKPds} \\ \hline
lausanne & \url{https://www.youtube.com/watch?v=GdhEsWcV4iE} \\ \hline
oxford & \url{https://www.youtube.com/watch?v=Qhq4vQdfrFw} \\ \hline
sittard & \url{https://www.youtube.com/watch?v=Zb9koIwo3Js} \\ \hline

\end{tabular}
\end{table}
